# Supplementary material for: Parallel Dynamic Spatial Indexes
Source: arXiv:2601.05347 source file (2026-01-08)
Supplement: Supplementary file 1 [file appendix-highdim-syn-table.tex]

% Table generated by Excel2LaTeX from sheet 'revis-summary-high-dim'
\begin{table*}[h]
	\centering
	\small
	\setlength\tabcolsep{6pt} % column width
	 % row width

	% Table generated by Excel2LaTeX from sheet 'revis-summary-high-dim'
	\begin{tabular}{cc|c|cccc|cccc|c|c}
		\toprule
		\textbf{Benchmark}                    & \multirow{2}[2]{*}{\textbf{Baselines}} & \multirow{2}[2]{*}{\textbf{Build}} & \multicolumn{4}{c|}{\textbf{Batch Insert}} & \multicolumn{4}{c|}{\textbf{Batch Delete}} & \textbf{10-NN }  & \textbf{Range Report}                                                                                                                                                                                 \\
		\textbf{(100M-12D)}                   &                                        &                                    & \textbf{0.01\%}                            & \textbf{0.1\%}                             & \textbf{1\%}     & \textbf{10\%}         & \textbf{0.01\%}  & \textbf{0.1\%}   & \textbf{1\%}     & \textbf{10\%}    & \boldmath{}\textbf{$10^7$ queries}\unboldmath{} & \boldmath{}\textbf{$10^4$ queries}\unboldmath{} \\
		\midrule
		\multirow{4}[2]{*}{\textbf{\uniform}} & Ours                                   & \underline{.938}                   & \underline{.001}                           & \underline{.003}                           & \underline{.017} & \underline{.115}      & \underline{.002} & \underline{.005} & \underline{.029} & \underline{.148} & \underline{51.4}                                & \underline{17.4}                                \\
		                                      & \logtree                               & 19.9                               & .013                                       & .017                                       & 4.09             & 4.22                  & .345             & .347             & .345             & .427             & t.o.                                            & s.f.                                            \\
		                                      & \bhltree                               & 14.4                               & 13.1                                       & 13.0                                       & 13.3             & 14.6                  & 10.9             & 11.1             & 11.4             & 13.1             & t.o.                                            & s.f.                                            \\
		                                      & \cgal                                  & 112                                & 164                                        & 168                                        & 157              & 171                   & .032             & .278             & 2.83             & 30.0             & 63.7                                            & 109                                             \\
		\midrule
		\multirow{4}[2]{*}{\textbf{\varden}}  & Ours                                   & \underline{1.07}                   & \underline{.002}                           & \underline{.004}                           & \underline{.025} & \underline{.269}      & \underline{.002} & \underline{.005} & \underline{.023} & \underline{.169} & .048                                            & \underline{10.5}                                \\
		                                      & \logtree                               & 19.7                               & .012                                       & .013                                       & 3.99             & 4.00                  & .342             & .349             & .346             & .427             & t.o.                                            & s.f.                                            \\
		                                      & \bhltree                               & 14.4                               & 12.8                                       & 12.7                                       & 12.8             & 14.1                  & 11.3             & 11.8             & 11.9             & 13.0             & t.o.                                            & s.f.                                            \\
		                                      & \cgal                                  & 46.7                               & 70.7                                       & 63.7                                       & 59.5             & 63.9                  & .003             & .032             & .452             & 4.82             & \underline{.046}                                & 114                                             \\
		\bottomrule
	\end{tabular}%

	\caption{
		\textbf{Running time (in seconds) for the \ourlib{} and other baselines on $10^8$ points in 12 dimensions. Lower is better.}
			The 10-NN queries $10^7$ points in parallel, and the range report contains $10^4$ rectangle range queries in parallel with output size $10^4$ to $10^6$.
			All queries searches the tree in serial.
			``t.o.'': time out after 600s.
			``s.f.'': segmentation fault.
	}
	\label{table:highdimsyn}%
\end{table*}%
