# Supplementary material for: Parallel Dynamic Spatial Indexes
Source: arXiv:2601.05347 source file (2026-01-08)
Supplement: Supplementary file 2 [file appendix-ood-table.tex]

% Table generated by Excel2LaTeX from sheet 'revis-ood'
\begin{table}[t]
	\centering
	\small
	\setlength\tabcolsep{2.4pt}

	% Table generated by Excel2LaTeX from sheet 'revis-ood'
	\begin{tabular}{c|c|ccc|ccc}
		\toprule
		\multirow{3}[2]{*}{\textbf{Tree}}     & \multirow{3}[2]{*}{\textbf{Baselines}} & \multicolumn{6}{c}{\textbf{Query points}}                                                                                                                    \\
		\cline{3-8}
		                                      &                                        & \multicolumn{3}{c|}{\textbf{\uniform}}    & \multicolumn{3}{c}{\textbf{\varden}}                                                                             \\
		                                      &                                        & \textbf{1-NN}                             & \textbf{10-NN}                       & \textbf{100-NN}  & \textbf{1-NN}    & \textbf{10-NN}   & \textbf{100-NN}  \\
		\midrule
		\multirow{4}[2]{*}{\textbf{\uniform}} & Ours                                   & \underline{.209}                          & \underline{.765}                     & \underline{2.66} & \underline{.086} & \underline{.162} & \underline{.774} \\
		                                      & \logtree{}                             & 2.43                                      & 4.48                                 & 16.9             & 1.21             & 2.00             & 15.7             \\
		                                      & \bhltree{}                             & .315                                      & 1.02                                 & 4.24             & .204             & .911             & 8.89             \\
		                                      & \cgal{}                                & .333                                      & 2.32                                 & 13.0             & .108             & .223             & 1.57             \\
		\midrule
		\multirow{4}[2]{*}{\textbf{\varden}}  & Ours                                   & \underline{.938}                          & \underline{1.71}                     & \underline{4.15} & \underline{.056} & \underline{.190} & \underline{.888} \\
		                                      & \logtree{}                             & t.o.                                      & t.o.                                 & t.o.             & 2.43             & 4.48             & 16.9             \\
		                                      & \bhltree{}                             & t.o.                                      & t.o.                                 & t.o.             & .315             & 1.02             & 4.24             \\
		                                      & \cgal{}                                & 1.68                                      & 3.07                                 & 7.80             & .083             & .219             & 1.28             \\
		\bottomrule
	\end{tabular}%

	\caption{
		\textbf{In-distribution and out-of-distribution \knn{} query time (in seconds) for \ourlib{} and other baselines on synthetic datasets with 3 dimensions. Lower is better.} The tree contains $10^9$ points, and the query points contains $10^7$ candidates. ``t.o.'': time out after 600s.}
	\label{table:ood}%

	\small
	\setlength\tabcolsep{2.4pt}
	
	\begin{tabular}{c|cc|cccc|cccc}
		\toprule
		\multirow{2}[2]{*}{\textbf{Bench.}}                                                                       & \multirow{2}[2]{*}{\textbf{Baselines}}                & \multirow{2}[2]{*}{{$\boldsymbol{\alpha}$}} & \multicolumn{4}{c|}{\textbf{Batch Insert (1\%)}} & \multicolumn{4}{c}{\textbf{Batch Delete (1\%)}}                                                                                                                   \\
&                                              &                              & \textbf{2}                                       & \textbf{3}                                      & \textbf{5}                & \textbf{9}                & \textbf{2}                & \textbf{3}                & \textbf{5}                & \textbf{9}                \\
		\midrule
		\multicolumn{1}{c|}{\multirow{6}[2]{*}{\begin{tabular}[c]{@{}c@{}}Uniform\\ 1000M\end{tabular}}} & \multicolumn{1}{c}{\multirow{3}[1]{*}{Ours}} & 0.03                         & 2.95                                    & 4.23                                   & 6.05             & 10.3             & 3.46             & 4.60             & 6.66             & 10.9             \\
		                                                                                                 &                                              & 0.1                          & .686                                    & .799                                   & 1.36             & 1.97             & .776             & .986             & 1.52             & 2.19             \\
		                                                                                                 &                                              & 0.3                          & \underline{.104}                        & \underline{.107}                       & \underline{.123} & \underline{.152} & \underline{.121} & \underline{.134} & \underline{.171} & \underline{.232} \\
		                                                                                                 & Log-tree                                     & -                            & 2.16                                    & 2.66                                   & 3.67             & 6.19             & .396             & .485             & 1.94             & 2.39             \\
		                                                                                                 & BHL-tree                                     & -                            & 31.4                                    & 40.3                                   & 57.1             & 103              & 30.9             & 39.3             & 68.7             & 114              \\
		                                                                                                 & CGAL                                         & -                            & 1660                                    & 1815                                   & 1863             & 2145             & 41.2             & 41.3             & 45.0             & 40.2             \\
		\midrule
		\multicolumn{1}{c|}{\multirow{6}[2]{*}{\begin{tabular}[c]{@{}c@{}}Varden\\ 1000M\end{tabular}}}  & \multicolumn{1}{c}{\multirow{3}[1]{*}{Ours}} & 0.03                         & 2.81                                    & 3.05                                   & 4.21             & 9.65             & 7.79             & 10.7             & 10.9             & 20.5             \\
		                                                                                                 &                                              & 0.1                          & .485                                    & .690                                   & .978             & 1.83             & 2.09             & 2.09             & 2.65             & 4.11             \\
		                                                                                                 &                                              & 0.3                          & \underline{.055}                        & \underline{.107}                       & \underline{.157} & \underline{.350} & \underline{.049} & \underline{.112} & \underline{.127} & \underline{.237} \\
		                                                                                                 & Log-tree                                     & -                            & 2.01                                    & 2.60                                   & 3.72             & 6.07             & 1.06             & 1.14             & 1.92             & 2.30             \\
		                                                                                                 & BHL-tree                                     & -                            & 29.4                                    & 39.1                                   & 57.3             & 102              & 29.0             & 38.4             & 67.0             & 123              \\
		                                                                                                 & CGAL                                         & -                            & 849                                     & 700                                    & 582              & 599              & 13.0             & 9.53             & 23.1             & 3.90             \\
		\bottomrule
	\end{tabular}%

	\caption{
		\textbf{Batch update time (in seconds) for \ourlib{} and other baselines on synthetic datasets with dimensions 2, 3, 5, and 9. Lower is better.} The tree contains $10^9$ points, and the batch contains $10^7$ points from the same distribution as the points in the tree. Parameter $\alpha$ is the imbalance ratio used in \ourlib{}.}
	\label{table:3inba}%
\end{table}%
