# Supplementary material for: Parallel Dynamic Spatial Indexes
Source: arXiv:2601.05347 source file (2026-01-08)
Supplement: Supplementary file 4 [file appendix-perf-hardware-table.tex]

\begin{table}[t]
	% \centering
	% \Huge
	% \resizebox{.48\textwidth}{!}{

	\small
	\setlength\tabcolsep{2.2pt}

	% Table generated by Excel2LaTeX from sheet 'revis-perf'
	\begin{tabular}{cc|ccccccc}
		\toprule
		                                                       & \textbf{Tree} & \textbf{CC(M)}      & \textbf{Inst(M)}   & \textbf{IPC}     & \textbf{CRs(M)} & \textbf{CMs(M)} & \textbf{BR(M)}    & \textbf{BMs(M)}  \\
		\midrule
		\multirow{2}[2]{*}{\begin{sideways}HT\end{sideways}}   & \ours{}       & 95,300              & 31,084             & .326             & 926             & 508             & 6,832             & 58.0             \\
		                                                       & \oursbb{}     & \underline{33,885}  & \underline{17,143} & \underline{.506} & \underline{245} & \underline{134} & \underline{2,279} & \underline{18.0} \\
		\midrule
		\multirow{2}[2]{*}{\begin{sideways}HH\end{sideways}}   & \ours{}       & 69,078              & 22,127             & .320             & 557             & 361             & 4,114             & 117              \\
		                                                       & \oursbb{}     & \underline{27,987}  & \underline{10,831} & \underline{.387} & \underline{242} & \underline{150} & \underline{1,636} & \underline{44.0} \\
		\midrule
		\multirow{2}[2]{*}{\begin{sideways}CHEM\end{sideways}} & \ours{}       & 243,014             & 65,919             & \underline{.271} & 1,662           & 1,450           & 14,318            & 170              \\
		                                                       & \oursbb{}     & \underline{139,701} & \underline{32,887} & .235             & \underline{954} & \underline{820} & \underline{6,583} & \underline{107}  \\
		\midrule
		\multirow{2}[2]{*}{\begin{sideways}GL\end{sideways}}   & \ours{}       & 71,844              & 21,767             & \underline{.303} & 439             & 345             & 3,376             & 118              \\
		                                                       & \oursbb{}     & \underline{62,637}  & \underline{13,438} & .215             & \underline{407} & \underline{317} & \underline{1,981} & \underline{101}  \\
		\midrule
		\multirow{2}[2]{*}{\begin{sideways}CM\end{sideways}}   & \ours{}       & \underline{120,478} & 22,407             & \underline{.186} & \underline{692} & \underline{649} & 3,397             & \underline{173}  \\
		                                                       & \oursbb{}     & 133,104             & \underline{21,913} & .165             & 752             & 703             & \underline{3,296} & 176              \\
		\midrule
		\multirow{2}[2]{*}{\begin{sideways}OSM\end{sideways}}  & \ours{}       & \underline{71,679}  & 12,247             & \underline{.171} & \underline{460} & \underline{426} & 1,366             & 50.0             \\
		                                                       & \oursbb{}     & 75,185              & \underline{11,124} & .148             & 473             & 441             & \underline{1,178} & \underline{48.0} \\
		\bottomrule
	\end{tabular}%

	% }
	\caption{
		\textbf{Hardware profiling of vanilla \ourlib{} (\ours{}) and a variant with bounding box optimizations (\oursbb{}) for range report query on real-world datasets.
			Underlined values indicate better performance.
		}
		The range report query contains $10^4$ rectangles each with output size $10^4$--$10^6$. Different queries are performed in parallel, and each query searches the tree in serial.
		``CC'': Cycles, ``Inst'': Instructions, ``IPC'': Instructions per cycle, ``CR'': Cache reference, ``CMs'': Cache misses, ``BR'': Branches, ``BMs'': Branch misses.
	}

	\label{table:appendix:perf-hardware}%

	\small
	\setlength\tabcolsep{6pt}
	
	\begin{tabular}{cc|ccccc}
		\toprule
		                                                       & \multirow{2}[2]{*}{\textbf{Tree}} & \multirow{2}[2]{*}{\textbf{Time (sec.)}} & \multicolumn{4}{c}{\textbf{Average \# of nodes proceed}}                                                            \\
		                                                       &                                   &                                          & \textbf{Leaf}                                            & \textbf{Interior} & \textbf{Skip}     & \textbf{Flatten} \\
		\midrule
		\multirow{2}[2]{*}{\begin{sideways}HT\end{sideways}}   & \ours{}                           & .587                                     & 2,675                                                    & 3,957             & \underline{1,282} & 0                \\
		                                                       & \oursbb{}                         & \underline{.268}                         & \underline{207}                                          & \underline{891}   & 605               & \underline{79}   \\
		\midrule
		\multirow{2}[2]{*}{\begin{sideways}HH\end{sideways}}   & \ours{}                           & .385                                     & 2,817                                                    & 3,621             & \underline{802}   & 3                \\
		                                                       & \oursbb{}                         & \underline{.192}                         & \underline{615}                                          & \underline{1,135} & 455               & \underline{65}   \\
		\midrule
		\multirow{2}[2]{*}{\begin{sideways}CHEM\end{sideways}} & \ours{}                           & 1.15                                     & 4,276                                                    & 5,701             & \underline{1,425} & 0                \\
		                                                       & \oursbb{}                         & \underline{.837}                         & \underline{1,330}                                        & \underline{2,506} & 1,091             & \underline{84}   \\
		\midrule
		\multirow{2}[2]{*}{\begin{sideways}GL\end{sideways}}   & \ours{}                           & .329                                     & 3,268                                                    & 5,478             & \underline{2,042} & 167              \\
		                                                       & \oursbb{}                         & \underline{.291}                         & \underline{1,285}                                        & \underline{3,484} & 1,993             & \underline{206}  \\
		\midrule
		\multirow{2}[2]{*}{\begin{sideways}CM\end{sideways}}   & \ours{}                           & \underline{.531}                         & 2,456                                                    & 3,939             & 1,053             & 429              \\
		                                                       & \oursbb{}                         & .577                                     & \underline{2,195}                                        & \underline{3,785} & \underline{1,120} & \underline{470}  \\
		\midrule
		\multirow{2}[2]{*}{\begin{sideways}OSM\end{sideways}}  & \ours{}                           & \underline{.326}                         & 529                                                      & 1,243             & 435               & 278              \\
		                                                       & \oursbb{}                         & .363                                     & \underline{236}                                          & \underline{959}   & \underline{439}   & \underline{284}  \\
		\bottomrule
	\end{tabular}%

	% }
	\caption{
		\textbf{Algorithmic statistic of vanilla \ourlib{} (\ours{}) and with bounding-box optimizations (\oursbb{}) for range report on real-world datasets. Underlined values indicate better performance.}
		The range report query contains $10^4$ rectangles each with output size $10^4$--$10^6$. Different queries are performed in parallel, and each query searches the tree in serial.
		``Leaf'': average number of leaf nodes visited per query, ``Interior'': average number of non-leaf nodes visited per query, ``Skip'': average number of nodes skipped per query, i.e., the associated sub-space does not intersect with the query box, ``Flatten'': average number of nodes flattened per query, i.e., the associated sub-space is fully contained in the query box.
	}
	\label{table:appendix:perf-alg}%
\end{table}%
