# Supplementary material for: Parallel Dynamic Spatial Indexes
Source: arXiv:2601.05347 source file (2026-01-08)
Supplement: Supplementary file 5 [file appendix-perf-mix-table.tex]

% \captionsetup{labelfont={bf, color=\revcolor}, textfont={color=\revcolor}}
\begin{table}[t]
	\centering
	% \Huge
	% \resizebox{.48\textwidth}{!}{

	\small
	\setlength\tabcolsep{3pt}

	% \color{\revcolor}

	% Table generated by Excel2LaTeX from sheet 'revis-perf'
	\begin{tabular}{cc|cccccc}
		\toprule
		                                                       & \textbf{Tree} & \textbf{Time(sec.)} & \textbf{\# Leaf}  & \textbf{\# Interior} & \textbf{IPC}     & \textbf{CRs(M)} & \textbf{CMs(M)} \\
		\midrule
		\multirow{2}[2]{*}{\begin{sideways}HT\end{sideways}}   & Pkd           & .587                & 2,675             & 3,957                & .326             & 926             & 508             \\
		                                                       & Pkd-bb        & \underline{.268}    & \underline{207}   & \underline{891}      & \underline{.506} & \underline{245} & \underline{134} \\
		\midrule
		\multirow{2}[2]{*}{\begin{sideways}HH\end{sideways}}   & Pkd           & .385                & 2,817             & 3,621                & .320             & 557             & 361             \\
		                                                       & Pkd-bb        & \underline{.192}    & \underline{615}   & \underline{1,135}    & \underline{.387} & \underline{242} & \underline{150} \\
		\midrule
		\multirow{2}[2]{*}{\begin{sideways}CHEM\end{sideways}} & Pkd           & 1.15                & 4,276             & 5,701                & \underline{.271} & 1,662           & 1,450           \\
		                                                       & Pkd-bb        & \underline{.837}    & \underline{1,330} & \underline{2,506}    & .235             & \underline{954} & \underline{820} \\
		\midrule
		\multirow{2}[2]{*}{\begin{sideways}GL\end{sideways}}   & Pkd           & .329                & 3,268             & 5,478                & \underline{.303} & 439             & 345             \\
		                                                       & Pkd-bb        & \underline{.291}    & \underline{1,285} & \underline{3,484}    & .215             & \underline{407} & \underline{317} \\
		\midrule
		\multirow{2}[2]{*}{\begin{sideways}CM\end{sideways}}   & Pkd           & \underline{.531}    & 2,456             & 3,939                & \underline{.186} & \underline{692} & \underline{649} \\
		                                                       & Pkd-bb        & .577                & \underline{2,195} & \underline{3,785}    & .165             & 752             & 703             \\
		\midrule
		\multirow{2}[2]{*}{\begin{sideways}OSM\end{sideways}}  & Pkd           & \underline{.326}    & 529               & 1,243                & \underline{.171} & \underline{460} & \underline{426} \\
		                                                       & Pkd-bb        & .363                & \underline{236}   & \underline{959}      & .148             & 473             & 441             \\
		\bottomrule
	\end{tabular}%

	% }
	\caption{
		\textbf{Performance comparison of the original \ourlib{} (Pkd) and a variant with bounding boxes (Pkd-bb) for range report queries on real-world datasets. The best performance is underlined.
		}
		The query contains $10^4$ range report queries with output size $10^4$--$10^6$.
		%Different queries are performed in parallel, and each query searches the tree in serial.
		``Time'': Time for all queries in seconds, ``Leaf'': Average number of leaf nodes visited per query, ``Interior'': Average number of interior nodes visited per query,
		``IPC'': Instructions per cycle, ``CR'': Cache reference, ``CMs'': Cache misses.
	}

	\label{table:perf-mix}%
\end{table}%
