# Supplementary material for: Parallel Dynamic Spatial Indexes
Source: arXiv:2601.05347 source file (2026-01-08)
Supplement: Supplementary file 6 [file appendix-rtree-zdtree-table.tex]

% Table generated by Excel2LaTeX from sheet 'Intro table'
\begin{table*}[t]
	\centering
	\small
	\setlength\tabcolsep{6pt} % column width
	 % row width

	% Table generated by Excel2LaTeX from sheet 'revis-rtree'
	\begin{tabular}{cc|c|cccc|cccc|c|c}
		\toprule
		\textbf{Benchmark}                    & \multirow{2}[2]{*}{\textbf{Baselines}} & \multirow{2}[2]{*}{\textbf{Build}} & \multicolumn{4}{c|}{\textbf{Batch Insert}} & \multicolumn{4}{c|}{\textbf{Batch Delete}} & \textbf{10-NN }  & \textbf{Range Report}                                                                                                                     \\
		\textbf{(1000M-2D)}                   &                                        &                                    & \textbf{0.01\%}                            & \textbf{0.1\%}                             & \textbf{1\%}     & \textbf{10\%}         & \textbf{0.01\%}  & \textbf{0.1\%}   & \textbf{1\%}     & \textbf{10\%}    & \textbf{(1\%)}   & \textbf{(10K, 1M]} \\
		\midrule
		\multirow{3}[2]{*}{\textbf{\uniform}} & Ours                                   & \underline{3.15}                   & \underline{.004}                           & \underline{.020}                           & \underline{.104} & \underline{.495}      & \underline{.004} & \underline{.022} & \underline{.121} & \underline{.526} & \underline{.381} & \underline{.391}   \\
		                                      & \rtree{} (seq.)                        & 363                                & .282                                       & 2.86                                       & 28.6             & 287                   & 1.10             & 11.6             & 121              & 1188             & 5.64             & 1.62               \\
		                                      & \zdtree                                & 6.70                               & n.a.                                       & n.a.                                       & n.a.             & n.a.                  & n.a.             & n.a.             & n.a.             & n.a.             & .870             & n.a.               \\
		\midrule
		\multirow{3}[2]{*}{\textbf{\varden}}  & Ours                                   & \underline{3.66}                   & \underline{.002}                           & \underline{.007}                           & \underline{.055} & \underline{.473}      & \underline{.002} & \underline{.006} & \underline{.049} & \underline{.477} & \underline{.172} & \underline{.382}   \\
		                                      & \rtree{} (seq.)                        & 336                                & .060                                       & .606                                       & 6.21             & 64.7                  & .267             & 2.23             & 24.7             & 308              & 1.79             & 1.60               \\
		                                      & \zdtree                                & 6.70                               & n.a.                                       & n.a.                                       & n.a.             & n.a.                  & n.a.             & n.a.             & n.a.             & n.a.             & .331             & n.a.               \\
		\bottomrule
	\end{tabular}%

	\vspace{.2em}
	\caption{
		\textbf{Running time (in seconds) for the \ourtree{} and other baselines on $10^9$ points in 2 dimensions. Lower is better.} \normalfont
		``\rtree{} (seq.)'': the serial \rtree{} implementation from Boost~\cite{schaling2011boost}.
		``\zdtree'': the parallel Quad/Oct-tree implementation using the Morton order from~\cite{blelloch2022parallel}.
		``10-NN'': 10-nearest-neighbor queries on $10^7$ points.
		``Range report'': orthogonal range report queries on $10^4$ rectangles, with output sizes in $10^4$--$10^6$.
		The fastest time for each test is underlined.
		``n.a.'': not applicable.
	}
	% \vspace{-1em}
	\label{table:app_rtree_zdtree}%
\end{table*}%
