# Supplementary material for: Parallel Dynamic Spatial Indexes
Source: arXiv:2601.05347 source file (2026-01-08)
Supplement: Supplementary file 9 [file appendix-rtree-table.tex]

% Table generated by Excel2LaTeX from sheet 'revis-rtree'
\begin{table}[t]
	\centering
	\small
	\setlength\tabcolsep{4pt}

	% Table generated by Excel2LaTeX from sheet 'revis-rtree'
	\begin{tabular}{cc|c|c|c}
		\toprule
		\textbf{Benchmark}                    & \multirow{2}[2]{*}{\textbf{Baselines}} & \multirow{2}[2]{*}{\textbf{Build}} & \textbf{10-NN }                                 & \textbf{Range Report}                           \\
		\textbf{(1000M-2D)}                   &                                        &                                    & \boldmath{}\textbf{$10^7$ queries}\unboldmath{} & \boldmath{}\textbf{$10^4$ queries}\unboldmath{} \\
		\midrule
		\multirow{2}[2]{*}{\textbf{\uniform}} & Ours                                   & \underline{3.15}                   & \underline{.381}                                & \underline{.391}                                \\
		                                      & \rtree                                 & 363                                & 5.64                                            & 1.62                                            \\
		\midrule
		\multirow{2}[2]{*}{\textbf{\varden}}  & Ours                                   & \underline{3.66}                   & \underline{.172}                                & \underline{.382}                                \\
		                                      & \rtree                                 & 336                                & 1.79                                            & 1.60                                            \\
		\bottomrule
	\end{tabular}%

	\caption{\textbf{Tree construction, \knn{} and range report on synthetic datasets for \ourlib{} and \rtree{}. Lower is better.} The \knn{} contains $10^7$ queries, and the range report queries $10^4$ rectangles, with out size in $10^4-10^6$.}
	\label{table:rtree}
\end{table}%
